# Supplementary material for: Deformable Sprites for Unsupervised Video Decomposition
Source: arXiv:2204.07151 source file (2022-04-14)
Supplement: Supplementary file 1 [file X_supplementary.tex]

\appendix

\setcounter{page}{1}

\twocolumn[
\centering
\Large{
\textbf{Deformable Sprites for Unsupervised Video Decomposition}
} \\
\vspace{0.5em}Supplementary Material \\
\vspace{1.0em}
] %
\appendix

\newcommand{\Ff}{F_{t\rightarrow t+1}}
\newcommand{\Fb}{F_{t+1 \rightarrow t}}

\paragraph{Parameterization of rigid transforms (Section 3.3)}
We parameterize the homography as a decomposed chain of transformations, as in \cite{hartley2003multiple}:
\begin{equation}
    \bf H = \begin{bmatrix}
    s \bf R & \bf t\\
    \bf 0^\top & 1\\
    \end{bmatrix}
    \begin{bmatrix}
    \bf K & \bf 0 \\
    \bf 0^\top & 1\\
    \end{bmatrix}
    \begin{bmatrix}
    \bf I & \bf 0\\
    \bf v^\top & v
    \end{bmatrix},
\end{equation}
where $\tf R  \in SO(2)$ and $\tf K$ is an upper triangular with $\det\tf K = 1$.
The parameters we optimize over are then 
$\eta =
[ s \tf R_{11}, s \tf R_{12}, 
\tf t_1 , \tf t_2 , 
\tf K_{11}, \tf K_{12},
\tf v_1, \tf v_2 ] \in \mathbb{R}^8$.
We find this parameterization to be more stable, and to favor explaining the motion with rigid scaling and translation rather than perspective and skew effects.

\paragraph{B-spline details (Section 3.3, Equations 2 and 3)}
The 1D B-spline basis functions of degree $d$, $B_d^{\text{1d}}i(z) \in [0, 1]^{d+1}$ are defined for over the unit interval $[0, 1]$.
We use the degree $d=2$ vector basis function $B_2^{\text{1d}}(z) \in [0, 1]^3$:
\begin{equation} 
B_2^{\text{1d}}(z) = \begin{bmatrix}
\frac{(1 - z)^2}{2}, & -z^2 + z + 0.5, & \frac{z^2}{2}
\end{bmatrix}^\top.
\end{equation}
In 2D, the degree $d=2$ basis functions $B_2^{\text{2d}}(u, v)$ are matrices in $[0, 1]^{3 \times 3}$
defined for $u, v \in [0, 1]$.
\begin{equation}
    B_2^{\text{2d}}(u, v) = B_2^{\text{1d}}(u) \cdot B_2^{\text{1d}}(v)^\top.
\end{equation}
For each interpolated query point, we blend the $d+1=3$ neighboring knot values (in each dimension) using the weights given by the respective basis functions.

\paragraph{Determining transform scales (Section 4)}
The transformations are optimized to be consistent with the optical flow in the coordinate space of the input images,
but the scale factor $s^{(\ell)}$ between each layer's sprite and the input images is not well-determined.
We determine the scale of each layer with the predicted masks after 5 epochs of training.
For each frame $t$ and layer $\ell$, we compute the mean flow, $\mu_t^{(\ell)} \in \mathbb{R}^2$ as in Equation 8, 
and the bounding box coordinates, $a_t^{(\ell)}, b_t^{(\ell)} \in \mathbb{R}^2$,
of the points $\{x;~M_t^{(\ell)(x)} \ge 0.5\}$.
The displacement of layer $\ell$ at time $t$ is $\delta_t^{(\ell)} = \sum_{\tau = 1}^t \mu_\tau^{(\ell)}$.
We estimate the total area covered by each layer from the start frame as a bounding box with minimum coordinate $\alpha^{(\ell)}$ and maximum coordinate $\beta_t^{(\ell)}$
\begin{equation}
    \alpha^{(\ell)} = \min_t\{a_t^{(\ell)} - \delta_t^{(\ell)}\}, ~~ \beta^{(\ell)} = \max_t\{a_t^{(\ell)} - \delta_t^{(\ell)}\}.
\end{equation}
We set the scale factor for layer $\ell$ to be $s^{(\ell)} = \frac{2}{\beta^{(\ell)} - \alpha^{(\ell)}}$.
We also update the rigid translation of layer $\ell$ at time $t$ to be $s^{(\ell)} \cdot (\delta_t^{(\ell)} - \alpha^{(\ell)}) - 1$.
$\alpha^{(\ell)}$ and $\beta^{(\ell)}$ are thus mapped to $(-1, -1)$ and $(1, 1)$, respectively.

\paragraph{Scale invariance in transform loss (Section 4, Equation 10)}
We divide the transform loss by the scale of the transform in Equation 10 to prevent the transforms from becoming degenerate (scaled to 0).
Our loss results in transforms with more stable scales.
Given the homography parameterization of $\eta =
[ s \tf R_{11}, s \tf R_{12}, 
\tf t_1 , \tf t_2 , 
\tf K_{11}, \tf K_{12},
\tf v_1, \tf v_2 ] \in \mathbb{R}^8$, we use $s = \sqrt{\eta_1^2 + \eta_2^2}$ as the scale.

\paragraph{Rejection of poorly-estimated fundamental matrices (Section 4)}
We use the optical flow vectors of all pixels in the input frame to estimate the fundamental matrix required for $\loss{static}$.
Because least median of squares regression can handle outliers consisting up to 50\% of the data, the estimated fundamental matrix captures the static geometry in the cases when background pixels comprise at least half of the frame.
However, we will encounter outlier percentages greater than 50\% when they do not.

To distinguish the two cases, we observe a difference in the distribution of residuals in the two cases.
Fitting a fundamental matrix to a moving object in its local reference frame will result in a fairly even residual distribution: we observe a modest residual on all points.
In comparison, fitting a fundamental matrix to a static element with moving outliers will result in a bimodal residual distribution: the static points have low residuals, while outlier moving points have high residuals.
We implement this distinction by rejecting estimates with a median error greater than 1 pixel.

\paragraph{Computing occlusions for optical flow consistency (Section 4)}
We enforce optical flow consistency, using the losses in equations 10 and 11, for all pixels that are not occluded.
We compute occlusion using the method described in \cite{sundaram2010dense}.
We consider all points $x$ in $I_t$. Under the forward flow field $\Ff$, $x$ is taken to $x' = \Ff(x)$.
Under the backward flow field $\Fb$, $x'$ is taken to $x'' = \Fb(x')$.
We consider all points $x$ such that 
\begin{equation}
    \| x'' - x \|^2  >  0.01 \cdot \big( \Ff(x)^2 + \Fb(x')^2 \big) + 1.5
\end{equation}
to be occluded, and the corresponding points $x''$ to be the occluders.
We call $\omega(I_t)$ the set of such occluded points $x$ in $I_t$;
we call $\Omega(I_t)$ the set of such occluded points $x''$ in $I_t$.

\paragraph{Network architectures}
We implement our model in PyTorch \cite{NEURIPS2019_9015}.
We use a standard UNet architecture \cite{ronneberger2015unet} for both the grouping model and the texture generator.
We provide the architecture we used for the results reported in the paper in Tables~\ref{tab:grouping_net} and~\ref{tab:texture_net}.
All convolutions are $3 \times 3$ with a stride and padding of 1.
All layers use a ReLU activation function.
All upsampling and pooling layers use a scale factor of 2.

\paragraph{Optimization}
We optimize our losses with a schedule.
Initially the relative weight of the grouping loss is greater than those of the transform and recon losses.
After 5 epochs, we reduce the grouping loss weight to 0.1 of the original weight.
We use $\lambda_{\text{recon}} = 1$, $\lambda_{\text{group}} = 1$, $\lambda_{\text{transform}} = 1$.
We use the Adam optimizer with learning rate $10^{-3}$.
We train each video with batch size 8 on an NVIDIA RTX 2080, for videos resized to $240 \times 426$ spatial resolution, for a total of 200 epochs.
For a video with 80 frames of this size, optimization takes around 30 minutes.

\begin{table}[h!]
    \centering
    \begin{tabular}{|c|c|c|c|}
    \hline
         & layer & in channels & out channels \\
    \hline
         1 & conv, BN, avg pool & 16 & 32 \\
         2 & conv, BN, avg pool & 32 & 64 \\
         3 & conv, BN, avg pool & 64 & 64\\
         4 & conv, BN, UP & 64 & 64\\
         5 & skip3, conv, BN, UP & 128 & 32\\
         6 & skip2, conv, BN, UP & 64 & 16 \\
    \hline
    \end{tabular}
    \caption{Network architecture for the grouping network. BN is batch norm, UP is bilinear upsample.}
    \label{tab:grouping_net}
    \vspace{-3mm}
\end{table}

\begin{table}[h!]
    \centering
    \begin{tabular}{|c|c|c|c|}
    \hline
         & layer & in channels & out channels \\
    \hline
         1 & conv, BN, avg pool & 16 & 32 \\
         2 & conv, BN, avg pool & 32 & 64 \\
         3 & conv, BN, avg pool & 64 & 128\\
         4 & conv, BN, avg pool & 128 & 128\\
         5 & conv, BN, UP & 128 & 128 \\
         6 & skip4, BN, UP & 256 & 64 \\
         7 & skip3, conv, BN, UP & 128 & 32\\
         8 & skip2, conv, BN, UP & 64 & 16 \\
    \hline
    \end{tabular}
    \caption{Network architecture for the texture generator. BN is batch norm, UP is bilinear upsample.}
    \label{tab:texture_net}
    \vspace{-3mm}
\end{table}
